# Supplementary material for: Universal Text Representation from BERT: An Empirical Study
Source: arXiv:1910.07973 source file (2019-10-23)
Supplement: Supplementary file 1 [file appendix.pdf]

# Universal Text Representation from BERT: An Empirical Study (Appendix)

Anonymous ACL submission

## A Sentence Embedding Performance of [CLS]-pooling BERT Activations

Table 1 presents the raw values of sentence embedding evaluation on downstream and probing tasks. The embeddings are extracted from different BERT layers using [CLS]-pooling.

| Dataset | Metric | Layer -1 | Layer -2 | Layer -3 | Layer -4 | Layer -5 | Layer -6 | Layer -7 | Layer -8 | Layer -9 | Layer -10 | Layer -11 | Layer -12 |
|---|---|---|---|---|---|---|---|---|---|---|---|---|---|
| STS12 | Pearson Average | 0.2758 | 0.2527 | 0.255 | 0.2631 | 0.2564 | 0.2874 | 0.3438 | 0.397 | 0.4337 | 0.2791 | 0.2835 | 0.1813 |
| STS13 | Pearson Average | 0.2252 | 0.1878 | 0.1854 | 0.1888 | 0.1715 | 0.1841 | 0.2471 | 0.3013 | 0.325 | 0.1582 | 0.1523 | 0.0864 |
| STS14 | Pearson Average | 0.2563 | 0.2765 | 0.2583 | 0.2599 | 0.2531 | 0.2796 | 0.3015 | 0.3846 | 0.4142 | 0.166 | 0.1905 | 0.1118 |
| STS15 | Pearson Average | 0.3211 | 0.3449 | 0.2931 | 0.2864 | 0.2705 | 0.3163 | 0.3112 | 0.3914 | 0.3941 | 0.1507 | 0.1947 | 0.1076 |
| STS16 | Pearson Average | 0.4269 | 0.4043 | 0.3625 | 0.3555 | 0.3367 | 0.3798 | 0.4572 | 0.5131 | 0.4939 | 0.1974 | 0.2272 | 0.0944 |
| MR | Accuracy | 81.75 | 81.14 | 79.64 | 79.15 | 76.02 | 71.48 | 66.49 | 68.35 | 65.99 | 62.8 | 63.73 | 53.95 |
| CR | Accuracy | 86.67 | 86.44 | 85.53 | 83.23 | 79.66 | 77.99 | 72 | 69.75 | 67.57 | 65.57 | 67.39 | 64.19 |
| MPQA | Accuracy | 87.34 | 87.58 | 87.22 | 88.06 | 85.53 | 85.76 | 85.57 | 85.15 | 83.93 | 82.89 | 81.71 | 81.3 |
| SUBJ | Accuracy | 94.96 | 94.93 | 94.24 | 94.22 | 94.08 | 93.6 | 93.54 | 92.62 | 90.1 | 88.34 | 89.2 | 80.21 |
| SST-Binary | Accuracy | 86.99 | 85.23 | 84.24 | 83.8 | 81.77 | 82.21 | 80.29 | 76.94 | 76.06 | 74.9 | 76.88 | 68.97 |
| SST-Finegrained | Accuracy | 46.06 | 44.66 | 42.81 | 40.9 | 42.76 | 40.81 | 42.31 | 39.59 | 35.79 | 34.52 | 38.55 | 32.71 |
| TREC | Accuracy | 89.6 | 89.2 | 84.2 | 87.6 | 86 | 87.4 | 82.4 | 81.8 | 75.4 | 72.2 | 75 | 66 |
| MRPC | F1 | 79.69 | 79.18 | 79.89 | 80.63 | 80.85 | 81.09 | 81.22 | 81.64 | 78.62 | 81.44 | 77.1 | 80.07 |
| SICK-Entailment | Accuracy | 65.52 | 70.27 | 72.44 | 73.29 | 71.26 | 72.58 | 73.74 | 72.3 | 75.85 | 74.61 | 68.54 | 68.58 |
| SICK-Relatedness | Pearson | 0.6964 | 0.6694 | 0.6447 | 0.6776 | 0.6630 | 0.6950 | 0.7651 | 0.7869 | 0.7889 | 0.7514 | 0.7407 | 0.7170 |
| STSBenchmark | Pearson | 0.5052 | 0.4100 | 0.4565 | 0.4803 | 0.4961 | 0.4995 | 0.5764 | 0.6577 | 0.6768 | 0.5421 | 0.5284 | 0.4806 |
| Length Classification | Accuracy | 59.9 | 62.3 | 66.6 | 63.5 | 69.6 | 72.4 | 72.6 | 83.3 | 85.5 | 89.6 | 89.6 | 84.9 |
| Word Content Classification | Accuracy | 31.5 | 20.3 | 12.4 | 11 | 6.7 | 12.9 | 8 | 10.5 | 9.8 | 1.7 | 2.1 | 0.5 |
| Depth Classification | Accuracy | 28.2 | 29.4 | 29.3 | 28.2 | 27.7 | 28.9 | 30.5 | 30.2 | 27.4 | 27.8 | 29.8 | 27.9 |
| Top Constituents Classification | Accuracy | 67.3 | 69 | 65.8 | 70.3 | 75.7 | 73.1 | 70.7 | 67 | 49.2 | 47.1 | 51 | 47.9 |
| Bigram Shift Classification | Accuracy | 86 | 85.4 | 85.3 | 85.2 | 80.5 | 78.8 | 80.3 | 78.9 | 64.2 | 51.3 | 51.2 | 50 |
| Tense Classification | Accuracy | 88.9 | 89.4 | 89.3 | 89 | 89.3 | 88.8 | 88.5 | 88 | 85.7 | 85.5 | 83.7 | 78 |
| Subj-number Classification | Accuracy | 81.2 | 83 | 84.2 | 86.2 | 85.5 | 85.5 | 85.7 | 82.1 | 79.5 | 78.8 | 79.7 | 72 |
| Obj-number Classification | Accuracy | 77.2 | 76.1 | 75.5 | 77.9 | 78.5 | 79.5 | 78.3 | 78 | 77.5 | 77.2 | 73.9 | 71.1 |
| Odd Man Out Classification | Accuracy | 62.6 | 62.4 | 61.8 | 60 | 60.6 | 58.6 | 58.9 | 55.6 | 55.5 | 53.7 | 51.2 | 49.9 |
| Co-Ordniation Inversion | Accuracy | 71.1 | 72.5 | 73.7 | 73.2 | 69.7 | 69.5 | 61.6 | 52.9 | 52.2 | 52.8 | 51.5 | 50 |

Table 1: Raw values of sentence embedding evaluation. Embeddings are extracted from a pre-trained BERT using [CLS]-pooling method. Layer -1 is the top encoder layer, layer -12 is the bottom layer. A logistic regression layer is added on top of the embeddings for each task classifier.

## B Sentence Embedding Performance of Mean-pooling BERT Activations

Figure 1 presents a heatmap plot of sentence embedding performance. Embeddings are extracted using Mean-pooling layer-wise BERT activation from a pre-trained BERT. Table 2 are the raw values of the evaluation.

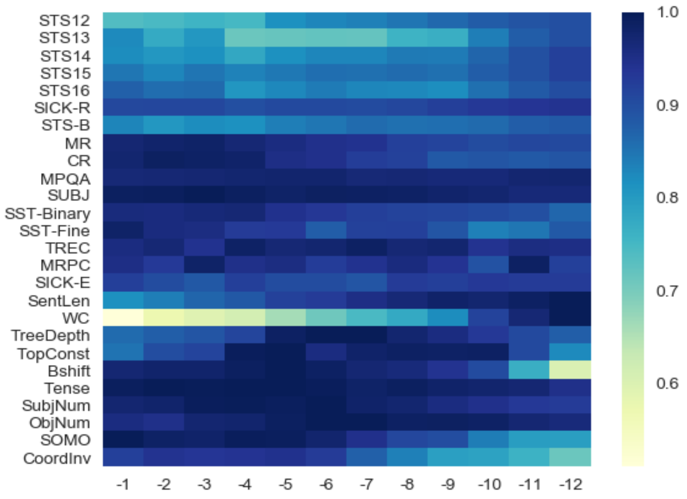


Figure 1: Sentence embedding performance of Mean-pooling layer-wise BERT activations. A color value of 1 corresponds to the best performance on a given task. Numbers on the x-axis represent the pooling layer with -1 being the top encoder layer, -12 being the bottom layer.

| Dataset | Metric | Layer -1 | Layer -2 | Layer -3 | Layer -4 | Layer -5 | Layer -6 | Layer -7 | Layer -8 | Layer -9 | Layer -10 | Layer -11 | Layer -12 |
|---|---|---|---|---|---|---|---|---|---|---|---|---|---|
| STS12 | Pearson Average | 0.4687 | 0.4729 | 0.4803 | 0.4754 | 0.5165 | 0.5258 | 0.5299 | 0.5391 | 0.5488 | 0.5588 | 0.5661 | 0.5705 |
| STS13 | Pearson Average | 0.5277 | 0.4956 | 0.5153 | 0.4566 | 0.459 | 0.4616 | 0.4605 | 0.4851 | 0.4901 | 0.5352 | 0.5615 | 0.5748 |
| STS14 | Pearson Average | 0.5715 | 0.5605 | 0.5668 | 0.5418 | 0.5673 | 0.5764 | 0.5765 | 0.5867 | 0.5857 | 0.6048 | 0.6246 | 0.6409 |
| STS15 | Pearson Average | 0.6347 | 0.6202 | 0.6353 | 0.6243 | 0.6329 | 0.6415 | 0.6401 | 0.6445 | 0.6396 | 0.6578 | 0.6712 | 0.6881 |
| STS16 | Pearson Average | 0.6451 | 0.6337 | 0.636 | 0.5954 | 0.609 | 0.6209 | 0.6112 | 0.6099 | 0.6038 | 0.631 | 0.6506 | 0.6651 |
| MR | Accuracy | 80.12 | 80.73 | 81.11 | 80.06 | 79.11 | 78.16 | 77.76 | 75.9 | 75.37 | 74.53 | 75.18 | 74.86 |
| CR | Accuracy | 85.83 | 86.94 | 86.73 | 86.25 | 83.84 | 83.37 | 81.24 | 80.71 | 77.75 | 78.31 | 77.8 | 78.28 |
| MPQA | Accuracy | 87.51 | 87.64 | 87.82 | 88.06 | 88.31 | 88.25 | 87.44 | 87.67 | 87.19 | 87.24 | 87.93 | 88.04 |
| SUBJ | Accuracy | 94.72 | 94.99 | 95.49 | 94.85 | 94.04 | 94.67 | 94.43 | 94.24 | 93.64 | 93.31 | 92.5 | 92.5 |
| SST-Binary | Accuracy | 85.17 | 85.01 | 85.45 | 85.83 | 83.53 | 82.54 | 81.6 | 81.05 | 80.72 | 80.18 | 79.52 | 76.66 |
| SST-Finegrained | Accuracy | 47.38 | 46.29 | 46.11 | 44.71 | 44.8 | 42.31 | 44.25 | 44.34 | 42.81 | 40.27 | 40.86 | 42.58 |
| TREC | Accuracy | 89.8 | 90.8 | 88.4 | 92.2 | 90.8 | 91.4 | 92.4 | 90.8 | 91.4 | 88.2 | 89.6 | 89.2 |
| MRPC | F1 | 79.26 | 77.27 | 81.69 | 78.91 | 79.5 | 77.01 | 78.39 | 79.8 | 78.05 | 74.25 | 82.01 | 76.54 |
| SICK-Entailment | Accuracy | 78.83 | 77.13 | 75.79 | 78.83 | 77.17 | 77.23 | 76.07 | 79.24 | 78.85 | 79.64 | 79.34 | 79.32 |
| SICK-Relatedness | Pearson | 0.8057 | 0.8076 | 0.8062 | 0.7972 | 0.8042 | 0.8037 | 0.8017 | 0.8076 | 0.8172 | 0.8248 | 0.8299 | 0.8345 |
| STSBenchmark | Pearson | 0.6540 | 0.6341 | 0.6463 | 0.6423 | 0.6604 | 0.6675 | 0.6784 | 0.6731 | 0.6760 | 0.6800 | 0.6915 | 0.6956 |
| Length Classification | Accuracy | 78.3 | 80.4 | 83.4 | 85 | 88.2 | 89.2 | 91.5 | 92.9 | 94.2 | 93.7 | 94.8 | 96 |
| Word Content Classification | Accuracy | 46.3 | 51.9 | 54.1 | 55.8 | 60.1 | 64.5 | 67.8 | 70.5 | 74.4 | 83.2 | 88 | 90.7 |
| Depth Classification | Accuracy | 33.4 | 34 | 34.5 | 35.4 | 38.3 | 38.8 | 38.8 | 37.9 | 37.2 | 36.2 | 35.2 | 34 |
| Top Constituents Classification | Accuracy | 65.5 | 69.3 | 70.3 | 76.6 | 76.9 | 73.7 | 75.5 | 76 | 75.8 | 76 | 69.7 | 63.4 |
| Bigram Shift Classification | Accuracy | 88.2 | 88.9 | 89 | 90.1 | 90.8 | 89.7 | 88.3 | 87.6 | 85.5 | 82.2 | 69.7 | 54.7 |
| Tense Classification | Accuracy | 88.8 | 89.3 | 89.2 | 89.4 | 89.3 | 88.9 | 88 | 88.7 | 87.7 | 87.5 | 87 | 84.9 |
| Subj-number Classification | Accuracy | 84.1 | 84.6 | 85.9 | 86 | 85.7 | 86.3 | 84.8 | 84.3 | 82.7 | 81.8 | 80.4 | 80.1 |
| Obj-number Classification | Accuracy | 81 | 80.2 | 82.2 | 82.5 | 83.7 | 84.4 | 84.4 | 83.4 | 83.5 | 83.2 | 82 | 81.4 |
| Odd Man Out Classification | Accuracy | 66 | 65 | 64.8 | 65.7 | 65.5 | 64.6 | 62.5 | 60.1 | 59.5 | 55.4 | 52.5 | 52.4 |
| Co-Ordniation Inversion | Accuracy | 67.9 | 69.4 | 69 | 69.2 | 69.7 | 68.4 | 64.4 | 61.6 | 58.4 | 58.1 | 56.2 | 52.6 |

Table 2: Raw values of sentence embedding evaluation. Embeddings are extracted from a pre-trained BERT using Mean-pooling method. Layer -1 is the top encoder layer, layer -12 is the bottom layer. A logistic regression layer is added on top of the embeddings for each task classifier.

## C Comparison Across Models

Table 3 presents the raw values of sentence embedding evaluation on downstream and probing tasks. The BERT sentence embeddings are extracted using Mean-pooling.

## D Statistics of Question-Answering Datasets

The basic statistics of the four question-answering datasets used in the experiments are presented in Table 4

| Dataset | Metric | PT (t) | MNLI (t) | SNLI (t) | PT (t+b) | MNLI (t+b) | SNLI (t+b) | GloVe | USE | InferSent |
|---|---|---|---|---|---|---|---|---|---|---|
| STS12 | Pearson Average | 0.4687 | 0.5602 | 0.6341 | 0.5466 | 0.591 | 0.63 | 0.5223 | 0.6257 | 0.6178 |
| STS13 | Pearson Average | 0.5277 | 0.5788 | 0.639 | 0.5736 | 0.6065 | 0.6351 | 0.496 | 0.6181 | 0.5596 |
| STS14 | Pearson Average | 0.5715 | 0.6384 | 0.6945 | 0.6313 | 0.6667 | 0.6916 | 0.546 | 0.695 | 0.6896 |
| STS15 | Pearson Average | 0.6347 | 0.6668 | 0.7012 | 0.6967 | 0.7207 | 0.7301 | 0.5626 | 0.748 | 0.724 |
| STS16 | Pearson | 0.6451 | 0.6558 | 0.6949 | 0.6848 | 0.6957 | 0.714 | 0.5141 | 0.737 | 0.717 |
| MR | Accuracy | 80.12 | 80.46 | 80.95 | 79.71 | 79.8 | 80.32 | 76.93 | 79.6 | 75.42 |
| CR | Accuracy | 85.83 | 87.63 | 86.46 | 86.41 | 86.73 | 85.43 | 78.36 | 85.3 | 82.44 |
| MPQA | Accuracy | 87.51 | 89.47 | 88.61 | 89.15 | 90 | 89.69 | 87.66 | 86.69 | 88.59 |
| SUBJ | Accuracy | 94.72 | 93.78 | 93.61 | 95.31 | 94.78 | 94.32 | 91.18 | 93.97 | 91.97 |
| SST-Binary | Accuracy | 85.17 | 85.72 | 86.49 | 86.05 | 87.1 | 87.86 | 79.68 | 86.71 | 83.69 |
| SST-Finegrained | Accuracy | 47.38 | 44.98 | 47.96 | 45.88 | 44.71 | 47.01 | 43.8 | 47.65 | 45.57 |
| TREC | Accuracy | 89.8 | 90.8 | 86.2 | 92 | 93.8 | 89.6 | 82.6 | 93.6 | 89.8 |
| MRPC | F1 | 79.26 | 79.35 | 82.77 | 76.79 | 81.52 | 81.77 | 81.69 | 79.23 | 81.1 |
| SICK-Entailment | Accuracy | 78.83 | 80.78 | 84.09 | 80.62 | 83.05 | 84.94 | 78.69 | 81.53 | 85.43 |
| SICK-Relatedness | Pearson | 0.8057 | 0.8153 | 0.8639 | 0.8516 | 0.8593 | 0.8830 | 0.7992 | 0.8686 | 0.8857 |
| STSBenchmark | Pearson | 0.6540 | 0.7030 | 0.7594 | 0.6903 | 0.7201 | 0.7510 | 0.6479 | 0.7874 | 0.7692 |
| Length Classification | Accuracy | 78.3 | 75.6 | 73.2 | 94.1 | 94.9 | 95.2 | 59.3 | 57.6 | 72.9 |
| Word Content Classification | Accuracy | 46.3 | 39.5 | 41.7 | 69.6 | 72.6 | 72.2 | 74.8 | 43.7 | 37.3 |
| Depth Classification | Accuracy | 33.4 | 33.5 | 32.7 | 35.6 | 36.2 | 36 | 30.2 | 26.7 | 32.6 |
| Top Constituents Classification | Accuracy | 65.5 | 61.4 | 61.9 | 71.5 | 67.8 | 69.5 | 61.5 | 62 | 69.2 |
| Bigram Shift Classification | Accuracy | 88.2 | 81.9 | 84.3 | 88.7 | 82 | 84.2 | 50 | 59.1 | 53.4 |
| Tense Classification | Accuracy | 88.8 | 88.1 | 86 | 89 | 88.2 | 87.2 | 83.7 | 86.5 | 86.7 |
| Subj-number Classification | Accuracy | 84.1 | 84.2 | 83.6 | 85.2 | 83.8 | 84.2 | 78 | 77.6 | 84.3 |
| Obj-number Classification | Accuracy | 81 | 81.2 | 81.1 | 82.9 | 83.3 | 83 | 76.5 | 75.1 | 79 |
| Odd Man Out Classification | Accuracy | 66 | 63.8 | 64.4 | 64.5 | 63.6 | 62.6 | 49.8 | 56.4 | 52.7 |
| Co-Ordniation Inversion | Accuracy | 67.9 | 68.3 | 68.3 | 68.2 | 67.1 | 67.7 | 53.6 | 59 | 63 |

Table 3: Comparison across models. “PT” stands for pre-trained BERT. “MNLI” and “SNLI” stand for BERT fine-tuned on MNLI, SNLI, representatively. Letters in parentheses represent BERT pooling layers. “t” means top layer, “b” means bottom layer. Mean-pooling is used for all BERT embedding extraction. Logistic regression layer is added on top of the embeddings.

| Dataset | WikiPassageQA | InsuranceQA | Quasar-t | SearchQA |
|---|---|---|---|---|
| Type | non-factoid | non-factoid | factoid | factoid |
| Number of Questions | 4,165 | 16,889 | 43,012 | 140,961 |
| Number of Answer Passages | 244,136 | 27,413 | 4.3 million | 7.5 million |
| Answers per Question | 59 | 500 | 100 | 50 |
| Avg. Answer Passage Length (tokens) | 133 | 67 | 100 | 100 |

Table 4: Statistics of question-answering datasets
