# Supplementary material for: Universal Text Representation from BERT: An Empirical Study
Source: arXiv:1910.07973 source file (2019-10-23)
Supplement: Supplementary file 2 [file acl2019_temp.tex]

%
% File acl2019.tex
%
%% Based on the style files for ACL 2018, NAACL 2018/19, which were
%% Based on the style files for ACL-2015, with some improvements
%%  taken from the NAACL-2016 style
%% Based on the style files for ACL-2014, which were, in turn,
%% based on ACL-2013, ACL-2012, ACL-2011, ACL-2010, ACL-IJCNLP-2009,
%% EACL-2009, IJCNLP-2008...
%% Based on the style files for EACL 2006 by 
%%e.agirre@ehu.es or Sergi.Balari@uab.es
%% and that of ACL 08 by Joakim Nivre and Noah Smith

\documentclass[11pt,a4paper]{article}
\usepackage[hyperref]{acl2019}
\usepackage{times}
\usepackage{latexsym}
\usepackage{graphicx}
\usepackage{amsmath}
\usepackage{booktabs}
\usepackage{multirow}
\usepackage{csquotes}

\usepackage{url}

%\aclfinalcopy % Uncomment this line for the final submission
%\def\aclpaperid{***} %  Enter the acl Paper ID here

%\setlength\titlebox{5cm}
% You can expand the titlebox if you need extra space
% to show all the authors. Please do not make the titlebox
% smaller than 5cm (the original size); we will check this
% in the camera-ready version and ask you to change it back.

\newcommand\BibTeX{B\textsc{ib}\TeX}

\title{Universal Text Representation from BERT: An Empirical Study \\
(Appendix)}


\author{First Author \\
  Affiliation / Address line 1 \\
  Affiliation / Address line 2 \\
  Affiliation / Address line 3 \\
  \texttt{email@domain} \\\And
  Second Author \\
  Affiliation / Address line 1 \\
  Affiliation / Address line 2 \\
  Affiliation / Address line 3 \\
  \texttt{email@domain} \\}

\date{}

\begin{document}
\maketitle

\appendix
\onecolumn

\section{Sentence Embedding Performance of [CLS]-pooling BERT Activations}

Table \ref{tab:cls} presents the raw values of sentence embedding evaluation on downstream and probing tasks.
The embeddings are extracted from different BERT layers using [CLS]-pooling. 

\begin{table*}[h]
\scalebox{0.52}{
\begin{tabular}{llcccccccccccc}
\toprule
\textbf{Dataset} & \textbf{Metric} & \textbf{Layer -1} & \textbf{Layer -2} & \textbf{Layer -3} & \textbf{Layer -4} & \textbf{Layer -5} & \textbf{Layer -6} & \textbf{Layer -7} & \textbf{Layer -8} & \textbf{Layer -9} & \textbf{Layer -10} & \textbf{Layer -11} & \textbf{Layer -12} \\ \hline
STS12	&	Pearson Average	&	0.2758	&	0.2527	&	0.255	&	0.2631	&	0.2564	&	0.2874	&	0.3438	&	0.397	&	0.4337	&	0.2791	&	0.2835	&	0.1813 \\
STS13	&	Pearson Average	&	0.2252	&	0.1878	&	0.1854	&	0.1888	&	0.1715	&	0.1841	&	0.2471	&	0.3013	&	0.325	&	0.1582	&	0.1523	&	0.0864 \\
STS14	&	Pearson Average	&	0.2563	&	0.2765	&	0.2583	&	0.2599	&	0.2531	&	0.2796	&	0.3015	&	0.3846	&	0.4142	&	0.166	&	0.1905	&	0.1118 \\
STS15	&	Pearson Average	&	0.3211	&	0.3449	&	0.2931	&	0.2864	&	0.2705	&	0.3163	&	0.3112	&	0.3914	&	0.3941	&	0.1507	&	0.1947	&	0.1076 \\
STS16	&	Pearson Average	&	0.4269	&	0.4043	&	0.3625	&	0.3555	&	0.3367	&	0.3798	&	0.4572	&	0.5131	&	0.4939	&	0.1974	&	0.2272	&	0.0944 \\
MR	&	Accuracy	&	81.75	&	81.14	&	79.64	&	79.15	&	76.02	&	71.48	&	66.49	&	68.35	&	65.99	&	62.8	&	63.73	&	53.95 \\
CR	&	Accuracy	&	86.67	&	86.44	&	85.53	&	83.23	&	79.66	&	77.99	&	72	&	69.75	&	67.57	&	65.57	&	67.39	&	64.19 \\
MPQA	&	Accuracy	&	87.34	&	87.58	&	87.22	&	88.06	&	85.53	&	85.76	&	85.57	&	85.15	&	83.93	&	82.89	&	81.71	&	81.3 \\
SUBJ	&	Accuracy	&	94.96	&	94.93	&	94.24	&	94.22	&	94.08	&	93.6	&	93.54	&	92.62	&	90.1	&	88.34	&	89.2	&	80.21 \\
SST-Binary	&	Accuracy	&	86.99	&	85.23	&	84.24	&	83.8	&	81.77	&	82.21	&	80.29	&	76.94	&	76.06	&	74.9	&	76.88	&	68.97 \\
SST-Finegrained	&	Accuracy	&	46.06	&	44.66	&	42.81	&	40.9	&	42.76	&	40.81	&	42.31	&	39.59	&	35.79	&	34.52	&	38.55	&	32.71 \\
TREC	&	Accuracy	&	89.6	&	89.2	&	84.2	&	87.6	&	86	&	87.4	&	82.4	&	81.8	&	75.4	&	72.2	&	75	&	66 \\
MRPC	&	F1	&	79.69	&	79.18	&	79.89	&	80.63	&	80.85	&	81.09	&	81.22	&	81.64	&	78.62	&	81.44	&	77.1	&	80.07 \\
SICK-Entailment	&	Accuracy	&	65.52	&	70.27	&	72.44	&	73.29	&	71.26	&	72.58	&	73.74	&	72.3	&	75.85	&	74.61	&	68.54	&	68.58 \\
SICK-Relatedness	&	Pearson	&	0.6964	&	0.6694	&	0.6447	&	0.6776	&	0.6630	&	0.6950	&	0.7651	&	0.7869	&	0.7889	&	0.7514	&	0.7407	&	0.7170 \\
STSBenchmark	&	Pearson	&	0.5052	&	0.4100	&	0.4565	&	0.4803	&	0.4961	&	0.4995	&	0.5764	&	0.6577	&	0.6768	&	0.5421	&	0.5284	&	0.4806 \\
Length Classification	&	Accuracy	&	59.9	&	62.3	&	66.6	&	63.5	&	69.6	&	72.4	&	72.6	&	83.3	&	85.5	&	89.6	&	89.6	&	84.9 \\
Word Content Classification	&	Accuracy	&	31.5	&	20.3	&	12.4	&	11	&	6.7	&	12.9	&	8	&	10.5	&	9.8	&	1.7	&	2.1	&	0.5 \\
Depth Classification	&	Accuracy	&	28.2	&	29.4	&	29.3	&	28.2	&	27.7	&	28.9	&	30.5	&	30.2	&	27.4	&	27.8	&	29.8	&	27.9 \\
Top Constituents Classification	&	Accuracy	&	67.3	&	69	&	65.8	&	70.3	&	75.7	&	73.1	&	70.7	&	67	&	49.2	&	47.1	&	51	&	47.9 \\
Bigram Shift Classification	&	Accuracy	&	86	&	85.4	&	85.3	&	85.2	&	80.5	&	78.8	&	80.3	&	78.9	&	64.2	&	51.3	&	51.2	&	50 \\
Tense Classification	&	Accuracy	&	88.9	&	89.4	&	89.3	&	89	&	89.3	&	88.8	&	88.5	&	88	&	85.7	&	85.5	&	83.7	&	78 \\
Subj-number Classification	&	Accuracy	&	81.2	&	83	&	84.2	&	86.2	&	85.5	&	85.5	&	85.7	&	82.1	&	79.5	&	78.8	&	79.7	&	72 \\
Obj-number Classification	&	Accuracy	&	77.2	&	76.1	&	75.5	&	77.9	&	78.5	&	79.5	&	78.3	&	78	&	77.5	&	77.2	&	73.9	&	71.1 \\
Odd Man Out Classification	&	Accuracy	&	62.6	&	62.4	&	61.8	&	60	&	60.6	&	58.6	&	58.9	&	55.6	&	55.5	&	53.7	&	51.2	&	49.9 \\
Co-Ordniation Inversion	&	Accuracy	&	71.1	&	72.5	&	73.7	&	73.2	&	69.7	&	69.5	&	61.6	&	52.9	&	52.2	&	52.8	&	51.5	&	50 \\
\bottomrule
\end{tabular}
}
\caption{Raw values of sentence embedding evaluation. Embeddings are extracted from a pre-trained BERT using [CLS]-pooling method. Layer -1 is the top encoder layer, layer -12 is the bottom layer. A logistic regression layer is added on top of the embeddings for each task classifier.}
\label{tab:cls}
\end{table*}


\section{Sentence Embedding Performance of Mean-pooling BERT Activations}

Figure \ref{fig:mean_pooling} presents a heatmap plot of sentence embedding performance.  Embeddings are extracted using Mean-pooling layer-wise BERT activation from a pre-trained BERT. 
Table \ref{tab:mean} are the raw values of the evaluation.

\begin{figure}[!htb]
	\centering
	\includegraphics[width=0.65\textwidth]{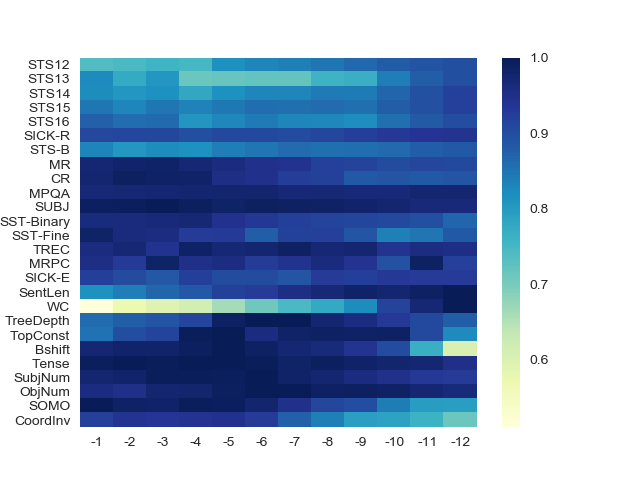}
	\caption{Sentence embedding performance of Mean-pooling layer-wise  BERT activations.  A color value of 1 corresponds to the best performance on a given task. Numbers on the x-axis represent the pooling layer with -1 being the top encoder layer, -12 being the bottom layer.}
	\label{fig:mean_pooling}
\end{figure}  


\begin{table*}[tbp]
\scalebox{0.52}{
\begin{tabular}{llcccccccccccc}
\toprule
\textbf{Dataset} & \textbf{Metric} & \textbf{Layer -1} & \textbf{Layer -2} & \textbf{Layer -3} & \textbf{Layer -4} & \textbf{Layer -5} & \textbf{Layer -6} & \textbf{Layer -7} & \textbf{Layer -8} & \textbf{Layer -9} & \textbf{Layer -10} & \textbf{Layer -11} & \textbf{Layer -12} \\ \hline
STS12	&	Pearson Average	&	0.4687	&	0.4729	&	0.4803	&	0.4754	&	0.5165	&	0.5258	&	0.5299	&	0.5391	&	0.5488	&	0.5588	&	0.5661	&	0.5705 \\
STS13	&	Pearson Average	&	0.5277	&	0.4956	&	0.5153	&	0.4566	&	0.459	&	0.4616	&	0.4605	&	0.4851	&	0.4901	&	0.5352	&	0.5615	&	0.5748 \\
STS14	&	Pearson Average	&	0.5715	&	0.5605	&	0.5668	&	0.5418	&	0.5673	&	0.5764	&	0.5765	&	0.5867	&	0.5857	&	0.6048	&	0.6246	&	0.6409 \\
STS15	&	Pearson Average	&	0.6347	&	0.6202	&	0.6353	&	0.6243	&	0.6329	&	0.6415	&	0.6401	&	0.6445	&	0.6396	&	0.6578	&	0.6712	&	0.6881 \\
STS16	&	Pearson Average	&	0.6451	&	0.6337	&	0.636	&	0.5954	&	0.609	&	0.6209	&	0.6112	&	0.6099	&	0.6038	&	0.631	&	0.6506	&	0.6651 \\
MR	&	Accuracy	&	80.12	&	80.73	&	81.11	&	80.06	&	79.11	&	78.16	&	77.76	&	75.9	&	75.37	&	74.53	&	75.18	&	74.86 \\
CR	&	Accuracy	&	85.83	&	86.94	&	86.73	&	86.25	&	83.84	&	83.37	&	81.24	&	80.71	&	77.75	&	78.31	&	77.8	&	78.28 \\
MPQA	&	Accuracy	&	87.51	&	87.64	&	87.82	&	88.06	&	88.31	&	88.25	&	87.44	&	87.67	&	87.19	&	87.24	&	87.93	&	88.04 \\
SUBJ	&	Accuracy	&	94.72	&	94.99	&	95.49	&	94.85	&	94.04	&	94.67	&	94.43	&	94.24	&	93.64	&	93.31	&	92.5	&	92.5 \\
SST-Binary	&	Accuracy	&	85.17	&	85.01	&	85.45	&	85.83	&	83.53	&	82.54	&	81.6	&	81.05	&	80.72	&	80.18	&	79.52	&	76.66 \\
SST-Finegrained	&	Accuracy	&	47.38	&	46.29	&	46.11	&	44.71	&	44.8	&	42.31	&	44.25	&	44.34	&	42.81	&	40.27	&	40.86	&	42.58 \\
TREC	&	Accuracy	&	89.8	&	90.8	&	88.4	&	92.2	&	90.8	&	91.4	&	92.4	&	90.8	&	91.4	&	88.2	&	89.6	&	89.2 \\
MRPC	&	F1	&	79.26	&	77.27	&	81.69	&	78.91	&	79.5	&	77.01	&	78.39	&	79.8	&	78.05	&	74.25	&	82.01	&	76.54 \\
SICK-Entailment	&	Accuracy	&	78.83	&	77.13	&	75.79	&	78.83	&	77.17	&	77.23	&	76.07	&	79.24	&	78.85	&	79.64	&	79.34	&	79.32 \\
SICK-Relatedness	&	Pearson	&	0.8057	&	0.8076	&	0.8062	&	0.7972	&	0.8042	&	0.8037	&	0.8017	&	0.8076	&	0.8172	&	0.8248	&	0.8299	&	0.8345 \\
STSBenchmark	&	Pearson	&	0.6540	&	0.6341	&	0.6463	&	0.6423	&	0.6604	&	0.6675	&	0.6784	&	0.6731	&	0.6760	&	0.6800	&	0.6915	&	0.6956 \\
Length Classification	&	Accuracy	&	78.3	&	80.4	&	83.4	&	85	&	88.2	&	89.2	&	91.5	&	92.9	&	94.2	&	93.7	&	94.8	&	96 \\
Word Content Classification	&	Accuracy	&	46.3	&	51.9	&	54.1	&	55.8	&	60.1	&	64.5	&	67.8	&	70.5	&	74.4	&	83.2	&	88	&	90.7 \\
Depth Classification	&	Accuracy	&	33.4	&	34	&	34.5	&	35.4	&	38.3	&	38.8	&	38.8	&	37.9	&	37.2	&	36.2	&	35.2	&	34 \\
Top Constituents Classification	&	Accuracy	&	65.5	&	69.3	&	70.3	&	76.6	&	76.9	&	73.7	&	75.5	&	76	&	75.8	&	76	&	69.7	&	63.4 \\
Bigram Shift Classification	&	Accuracy	&	88.2	&	88.9	&	89	&	90.1	&	90.8	&	89.7	&	88.3	&	87.6	&	85.5	&	82.2	&	69.7	&	54.7 \\
Tense Classification	&	Accuracy	&	88.8	&	89.3	&	89.2	&	89.4	&	89.3	&	88.9	&	88	&	88.7	&	87.7	&	87.5	&	87	&	84.9 \\
Subj-number Classification	&	Accuracy	&	84.1	&	84.6	&	85.9	&	86	&	85.7	&	86.3	&	84.8	&	84.3	&	82.7	&	81.8	&	80.4	&	80.1 \\
Obj-number Classification	&	Accuracy	&	81	&	80.2	&	82.2	&	82.5	&	83.7	&	84.4	&	84.4	&	83.4	&	83.5	&	83.2	&	82	&	81.4 \\
Odd Man Out Classification	&	Accuracy	&	66	&	65	&	64.8	&	65.7	&	65.5	&	64.6	&	62.5	&	60.1	&	59.5	&	55.4	&	52.5	&	52.4 \\
Co-Ordniation Inversion	&	Accuracy	&	67.9	&	69.4	&	69	&	69.2	&	69.7	&	68.4	&	64.4	&	61.6	&	58.4	&	58.1	&	56.2	&	52.6 \\

\bottomrule
\end{tabular}
}
\caption{Raw values of sentence embedding evaluation. Embeddings are extracted from a pre-trained BERT using Mean-pooling method. Layer -1 is the top encoder layer, layer -12 is the bottom layer. A logistic regression layer is added on top of the embeddings for each task classifier.}
\label{tab:mean}
\end{table*}


\section{Comparison Across Models}
Table \ref{tab:all_models} presents the raw values of sentence embedding evaluation on downstream and probing tasks.
The BERT sentence embeddings are extracted using Mean-pooling.

\begin{table*}[tbp]
\scalebox{0.63}{
\begin{tabular}{llccccccccc}
\toprule
\textbf{Dataset} & \textbf{Metric} & \textbf{PT (t)} & \textbf{MNLI (t)} & \textbf{SNLI (t)}  & \textbf{PT (t+b)} & \textbf{MNLI (t+b)} & \textbf{SNLI (t+b)} & \textbf{GloVe} & \textbf{USE} & \textbf{InferSent} \\ \hline
STS12	&	Pearson Average	&	0.4687	&	0.5602	&	0.6341	&	0.5466	&	0.591	&	0.63	&	0.5223	&	0.6257	&	0.6178 \\
STS13	&	Pearson Average	&	0.5277	&	0.5788	&	0.639	&	0.5736	&	0.6065	&	0.6351	&	0.496	&	0.6181	&	0.5596 \\
STS14	&	Pearson Average	&	0.5715	&	0.6384	&	0.6945	&	0.6313	&	0.6667	&	0.6916	&	0.546	&	0.695	&	0.6896 \\
STS15	&	Pearson Average	&	0.6347	&	0.6668	&	0.7012	&	0.6967	&	0.7207	&	0.7301	&	0.5626	&	0.748	&	0.724 \\
STS16	&	Pearson	&	0.6451	&	0.6558	&	0.6949	&	0.6848	&	0.6957	&	0.714	&	0.5141	&	0.737	&	0.717 \\
MR	&	Accuracy	&	80.12	&	80.46	&	80.95	&	79.71	&	79.8	&	80.32	&	76.93	&	79.6	&	75.42 \\
CR	&	Accuracy	&	85.83	&	87.63	&	86.46	&	86.41	&	86.73	&	85.43	&	78.36	&	85.3	&	82.44 \\
MPQA	&	Accuracy	&	87.51	&	89.47	&	88.61	&	89.15	&	90	&	89.69	&	87.66	&	86.69	&	88.59 \\
SUBJ	&	Accuracy	&	94.72	&	93.78	&	93.61	&	95.31	&	94.78	&	94.32	&	91.18	&	93.97	&	91.97 \\
SST-Binary	&	Accuracy	&	85.17	&	85.72	&	86.49	&	86.05	&	87.1	&	87.86	&	79.68	&	86.71	&	83.69 \\
SST-Finegrained	&	Accuracy	&	47.38	&	44.98	&	47.96	&	45.88	&	44.71	&	47.01	&	43.8	&	47.65	&	45.57 \\
TREC	&	Accuracy	&	89.8	&	90.8	&	86.2	&	92	&	93.8	&	89.6	&	82.6	&	93.6	&	89.8 \\
MRPC	&	F1	&	79.26	&	79.35	&	82.77	&	76.79	&	81.52	&	81.77	&	81.69	&	79.23	&	81.1 \\
SICK-Entailment	&	Accuracy	&	78.83	&	80.78	&	84.09	&	80.62	&	83.05	&	84.94	&	78.69	&	81.53	&	85.43 \\
SICK-Relatedness	&	Pearson	&	0.8057	&	0.8153	&	0.8639	&	0.8516	&	0.8593	&	0.8830	&	0.7992	&	0.8686	&	0.8857 \\
STSBenchmark	&	Pearson	&	0.6540	&	0.7030	&	0.7594	&	0.6903	&	0.7201	&	0.7510	&	0.6479	&	0.7874	&	0.7692 \\
Length Classification	&	Accuracy	&	78.3	&	75.6	&	73.2	&	94.1	&	94.9	&	95.2	&	59.3	&	57.6	&	72.9 \\
Word Content Classification	&	Accuracy	&	46.3	&	39.5	&	41.7	&	69.6	&	72.6	&	72.2	&	74.8	&	43.7	&	37.3 \\
Depth Classification	&	Accuracy	&	33.4	&	33.5	&	32.7	&	35.6	&	36.2	&	36	&	30.2	&	26.7	&	32.6 \\
Top Constituents Classification	&	Accuracy	&	65.5	&	61.4	&	61.9	&	71.5	&	67.8	&	69.5	&	61.5	&	62	&	69.2 \\
Bigram Shift Classification	&	Accuracy	&	88.2	&	81.9	&	84.3	&	88.7	&	82	&	84.2	&	50	&	59.1	&	53.4 \\
Tense Classification	&	Accuracy	&	88.8	&	88.1	&	86	&	89	&	88.2	&	87.2	&	83.7	&	86.5	&	86.7 \\
Subj-number Classification	&	Accuracy	&	84.1	&	84.2	&	83.6	&	85.2	&	83.8	&	84.2	&	78	&	77.6	&	84.3 \\
Obj-number Classification	&	Accuracy	&	81	&	81.2	&	81.1	&	82.9	&	83.3	&	83	&	76.5	&	75.1	&	79 \\
Odd Man Out Classification	&	Accuracy	&	66	&	63.8	&	64.4	&	64.5	&	63.6	&	62.6	&	49.8	&	56.4	&	52.7 \\
Co-Ordniation Inversion	&	Accuracy	&	67.9	&	68.3	&	68.3	&	68.2	&	67.1	&	67.7	&	53.6	&	59	&	63 \\
\bottomrule
\end{tabular}
}
\caption{Comparison across models. \enquote{PT} stands for pre-trained BERT. \enquote{MNLI} and \enquote{SNLI} stand for BERT fine-tuned on MNLI, SNLI, representatively. Letters in parentheses represent BERT pooling layers. \enquote{t} means top layer, \enquote{b} means bottom layer. Mean-pooling is used for all BERT embedding extraction. Logistic regression layer is added on top of the embeddings.}
\label{tab:all_models}
\end{table*}

\section{Statistics of Question-Answering Datasets}

The basic statistics of the four question-answering datasets used in the experiments are presented in Table \ref{tab:stats}

\begin{table}[tbp]
\scalebox{0.9}{
\begin{tabular}{lllll}
\bottomrule
\textbf{Dataset} & \textbf{WikiPassageQA} & \textbf{InsuranceQA} & \textbf{Quasar-t} & \textbf{SearchQA} \\ \hline
Type & non-factoid & non-factoid & factoid & factoid \\
Number of Questions & 4,165 & 16,889 & 43,012 & 140,961 \\
Number of Answer Passages & 244,136 & 27,413 & 4.3 million & 7.5 million\\
Answers per Question & 59 & 500 & 100 & 50 \\
Avg. Answer Passage Length (tokens) & 133 & 67 & 100 & 100 \\
\bottomrule
\end{tabular}
}
\caption{Statistics of question-answering datasets}
\label{tab:stats}
\end{table}


\end{document}
